# Supplementary material for: GPSfM: Global Projective SFM Using Algebraic Constraints on Multi-View Fundamental Matrices
Source: arXiv:1812.00426 source file (2021-06-06)
Supplement: Supplementary file 1 [file additionalLemma.tex]

\documentclass{article}

\usepackage{times}
\usepackage{epsfig}
\usepackage{graphicx}
\usepackage{amsmath}
\usepackage{amssymb}

\usepackage{comment}
\usepackage{caption}
\usepackage{wasysym}
\usepackage{amsthm}
\usepackage{color}
\usepackage{float}
\usepackage{multirow}
\usepackage{graphics}
\usepackage[english]{babel}

\newtheorem{theorem}{Theorem}[]
\newtheorem{corollary}{Corollary}[]
\newtheorem{lemma}[theorem]{Lemma}

\begin{document}

%In the following lemma we will show the version of the composition rule proved in [Alessandro Rudi] to the case of the n-view fundamental matrix
\begin{lemma} 
Let $F$ be a n-view matrix. Let $F^1,F^2$ be two sub-matrices of $F$ which contain together all the views in $F$ and are consistent multi-view matrices respectively. Then, if $F^1,F^2$ share at least one fundamental matrix $F_{ij}$, then $F^1,F^2$ uniquely define scale factors and completion for $F$ which is consistent. 
%option2: If two n-view matrices \(F^{1},F^2\) are consistent and there exist two shared views $i_1,i_2$ such that the corresponding fundamental coincide in $F^1,F^2$ than there  exists a unique n-view fundamental matrix \(F\) that agrees with both \(F^{1}\) and \(F^2\). This construction is error free.
\end{lemma}
\begin{proof}
By definition 2 $F^1,F^2$ define two sets of camera matrices $P^1,P^2$ that are compatible w.r.t them. It follows that there are two camera matrices in each set that are compatible with $F_{ij}$ and hence the two pairs are equal up to a projective homography [HZ]. As a result $P^1 $ can be transferred to the projective frame of $P^2 $ to form a set of $n$ camera matrices that are compatible with both $F^1,F^2$ [Alessandro Rudi].  %defines uniqely Then, by using [Alessandro Rudi] and the fact that \(F_{i_{1}i_2}^1=F_{i_{1}i_2}^2\) it holds that those two sets of camera matrices can be transformed by homography into one consistent set. Since $F^1,F^2$ are both consistent and agree on two views this transformation is error free. 
The consistent n-view matrix that is generated from these  cameras  form a unique (up to global $n$ scale factors) completion and re-scaling of $F$. %(since homographty doesn't change the fundamental matrices) and of course consistent.
\end{proof}
\begin{corollary}
Let $F$ be a n-view matrix. Then a set of consistent multi-view matrices \(F^{1},F^2,\dots,F^k\) which contain together all the views in $F$ such that each pair \(F^i,F^{i+1}\) share a fundamental matrix, uniquely define scale factors and completion for $F$ which is consistent
\end{corollary}
\begin{proof}
By induction over $k$. For $k=2$ it follows directly from Lemma 1.
Assume that the argument is true for $k-1$ and prove for $k$. 
By induction assumption it follows that \(F^{1},F^2,\dots,F^{k-1}\) defines uniquely a completion and scale factors for a consistent multi-view matrix $F^0$ which is a sub matrix of $F$ of all the views of \(F^{1},F^2,\dots,F^{k-1}\). Now $F^0$ and $F^k$ are consistent multi-view matrix and  share one fundamental matrix, and contain together all the views of $F$, by Lemma 1  they uniquely define scale factors and completion for $F$ which is consistent.       
\end{proof}
%[Alessandro Rudi] showed that two solved viewing graphs \(\gamma_1.\gamma_2\) that share two views can be composed into a bigger graph that agree with  \(\gamma_1.\gamma_2\) . 
\end{document}
