# Supplementary material for: GPSfM: Global Projective SFM Using Algebraic Constraints on Multi-View Fundamental Matrices
Source: arXiv:1812.00426 source file (2021-06-06)
Supplement: Supplementary file 2 [file appendix.tex]

Next we prove the following supporting lemmas for  Theorem \ref{thm:consistent_direct}. The first lemma, Lemma~\ref{lemma:consistent}, was introduced and proved in \cite{sengupta2017new}.

\setcounter{theorem}{0}

\begin{lemma}\label{lemma:consistent} \cite{sengupta2017new}  Let $F$ be a consistent $n$-view fundamental matrix. Then, 
\begin{enumerate}
\item 
$F$ can be formulated as $F=UV^{T}+VU^{T}$, where $V,U \in \Real^{3n \times 3}$ consist of $n$ blocks of size $3 \times 3$ 
\begin{align*}
V =\left[\begin{array}{ccc}
V_{1}\\
\vdots\\
V_{n}
\end{array}\right] ~~ & ~~
U =\left[\begin{array}{c}
V_{1} T_{1}\\
\vdots\\
V_{n} T_{n}
\end{array}\right]
\end{align*}
with $T_i = [{\bf t}_i]_{\times}$.
\item  $rank(V) = 3$ 
\item If not all ${\bf t}_i$ are collinear then $rank(U)=3$ and $rank(F) = 6$. 
\end{enumerate}
\end{lemma}

\begin{proof}
The first result is directly from the definition of consistency. Since $V_i$ is invertible for all $i=1, \ldots, n$, then $rank(V_i) =3$ and thus $rank(V) =3$. Next we show that under the assumption that not all ${\bf t}_i$ are collinear then $rank(U) =3$. We prove this by contradiction. Assume $rank(U) < 3$. Then, $\exists {\bf t} \neq 0$, s.t. $U {\bf t}=0$. Since $V_i$ are of full rank for all $i=1, \ldots, n$, this implies that ${\bf t}_i \times t = 0$ for all $i=1, \ldots, n$. Thus, all the ${\bf t}_i$'s are parallel to $t$ violating our assumption that not all ${\bf t}_i$ are collinear. We still need to show that under the assumption that not all ${\bf t}_i$ are collinear then $rank(F)=6$. Using the QR decomposition for an invertible matrix, each $V_i$ can be decomposed uniquely into a product of a  lower triangular matrix with positive diagonal elements and orthogonal matrix, i.e., there exist  an upper triangular $K_i$ and an orthogonal matrix $R_i$ such that $V_i = K_i^{-T} R_i^T$. This decomposition allows to complete the proof as described in the paper \cite{sengupta2017new}.
\end{proof}

\label{section::sufficient_conditions}
\begin{lemma}\label{lemma:eigenvalues}
Let $F \in S^{3n}$ be a matrix of rank 6. 
$F$ can be decomposed into $F=UV^{T}+VU^{T}$ with $U, V \in \Real^{3n\times3}$  $\Leftrightarrow$ $F$ has 3 positive and 3 negative eigenvalues.
\end{lemma}
\begin{proof} $\Leftarrow$ Assume that $F$ has 3 positive and
3 negative eigenvalues, which we denote by $\lambda_1 \geq \lambda_2 \geq \lambda_3 > 0 > \lambda_4 \geq \lambda_5 \geq \lambda_6$. Then,  by spectral decomposition of a symmetric matrix
\begin{align*}
F & =[\tilde{X},\tilde{Y}]\left(\begin{array}{cc}
\Sigma_{1} & 0\\
0 & -\Sigma_{2}
\end{array}\right)[\tilde{X},\tilde{Y}]^{T} \\
&=\tilde{X}\Sigma_{1}\tilde{X}^{T}-\tilde{Y}\Sigma_{2}\tilde{Y}^{T}
\end{align*}
where $\tilde{X}, \tilde{Y} \in \Real^{3n \times 3}$, $\Sigma_1 = \text{diag}(\lambda_1, \lambda_2, \lambda_3)$ and $\Sigma_2 = \text{diag}(-\lambda_4,- \lambda_5,- \lambda_6)$.  
Next, we define $X = \tilde{X} \sqrt{\Sigma_1}$ and $Y = \tilde{Y} \sqrt{\Sigma_2}$ then 
\begin{align*}
F & = XX^{T}-YY^{T} \\
& =\frac{1}{2}(X+Y)(X-Y)^{T}+\frac{1}{2}(X-Y)(X+Y)^{T}.
%& = UV^{T}+VU^{T}
\end{align*}
Now, we define $U=\sqrt{\frac{1}{2}}(X+Y)$ and $V=\sqrt{\frac{1}{2}}(X-Y)$ yielding the requested decomposition $F=UV^{T}+VU^{T}$. Note that this means that $F$ can be formulated as the symmetric part of the $3n \times 3n$ matrix $A=UV^T$, i.e., $F = A + A^T$, such that $\text{rank}(A) \leq 3$.

$\Rightarrow$ Assume that $F=UV^{T}+VU^{T}$, where $U, V \in \Real^{3n\times3}$. Now, we define  $X=\sqrt{\frac{1}{2}}(U+V)$ and $Y=\sqrt{\frac{1}{2}}(U-V)$ yielding  $F=XX^{T}-YY^{T}$.
 
 Since $F$ is symmetric of degree 6, it has exactly 6 real eigenvalues different from 0. We would like to show that $F$ has exactly 3 positive eigenvalues and 3 negative eigenvalues.  By contradiction,
w.l.o.g. assume that $F$ has at least 4  positive eigenvalues which we will
denote by $\lambda_{1},\lambda_{2},\lambda_{3},\lambda_{4}$ and their
corresponding eigenvectors by $v_{1},v_{2},v_{3},v_{4}$. Let denote the subspace spanned by these eigenvectors by $S$, i.e., $S =span\{v_{1},v_{2},v_{3},v_{4}\} $.

Now for every $\sum_{i=1}^{4} a_{i}v_{i}=z\in S$
we have due to orthogonality $$Fz = \sum_{i=1}^4 \alpha_i \lambda_i v_i  \Rightarrow z^T Fz= \sum_{i=1}^4 \alpha_i^2 \lambda_i.$$  Therefore, since $\lambda_i > 0$, for $0 \neq z \in S$ we have,  $$z^T F z = \sum_{i=1}^4 \alpha_i^2 \lambda_i > 0.$$
On the other hand, the dimension of the column space of $X$ is at most 3 and therefore  $\exists z \in S$, which is orthogonal to the column space of $X$, i.e. $X^Tz=0$, implying that
\begin{equation*}
z^T F z = z^T (X X^T - Y Y^T)z = - z^T Y Y^T z \leq 0,
\end{equation*}
which contradicts our previous observation that every vector $0 \neq z\in S$
satisfies $z^{T}Fz>0$.
 The same argument can be applied to the negative
eigenvalues. We conclude  that $F$ has exactly 3 positive eigenvalues and 3 negative eigenvalues.
\end{proof}

\begin{corollary}\label{Corollary 2.2} 
$F \in S^{k}$ of rank 6 with 3 positive and 3 negative eigenvalues can be formulated  as $F=UV^{T}+VU^{T}$, where $U, V \in \Real^{k\times3}$  
\end{corollary}
\yk{What is k? do we mean 3n? It was not defined above}

\begin{lemma}\label{lemma:common_null_space} Let $A,B\in \Real^{3\times3}$such that $rank(A)=rank(B)=2$
and $AB^{T}=[\bf{t}]_{\times}$ for some ${\bf t}\in \Real^{3}$ then $A^{T}{\bf t}=B^{T}{\bf t}=0$
\end{lemma}

\begin{proof}
Let have $0 \neq {\bf t}_1 \in Ker(A^T), 0 \neq {\bf t}_2 \in Ker(B^T)$. 

First  $AB^T = [\bf{t}]_{\times}$ implies $BA^T = - [{\bf t}]_{\times}$. Then,
$$A^T {\bf t}_1 = 0 \Rightarrow BA^T {\bf t}_1 = 0 \Rightarrow {\bf -t} \times {\bf t}_1 = 0 \Rightarrow {\bf t}_1 \parallel {\bf t} \Rightarrow A^T {\bf t} = 0$$
$$B^T {\bf t}_2 = 0 \Rightarrow AB^T {\bf t}_2 = 0 \Rightarrow {\bf t} \times {\bf t}_2 = 0 \Rightarrow {\bf t}_2 \parallel {\bf t} \Rightarrow B^T {\bf t} = 0$$
\end{proof}

\begin{lemma}\label{lemma:skew} Let $A,B\in \Real^{3\times3}$ with $rank(A)=2,\,\,rank(B)=3$
and $AB^{T}$ is skew symmetric (that is $AB^{T}+BA^{T}=0$) , then
$T=B^{-1}A$ is skew symmetric.
\end{lemma}

\begin{proof} Since $AB^{T}$ is skew symmetric it can be written 
as  $AB^{T}=[a]_{\times}$ for some $a\in \Real^{3}\Rightarrow$
\begin{align*}
A=[a]_{\times}B^{-T}=BB^{-1}[a]_{\times}B^{-T}=B(B^{-1}[a]_{\times}B^{-T})=B\frac{[B^{T}a]_{\times}}{det(B)} \end{align*}
where the last equality follows from Lemma \ref{lemma:identity}. \rb{correct reference}
Consequently, $T=B^{-1}A=\frac{[B^{T}a]_{\times}}{det(B)}$ is skew symmetric.

\end{proof}

\begin{lemma}\label{lemma:xor}
Let $U, V \in \Real^{3n \times 3}$ and respectively denote their $3 \times 3$ blocks by $U_i$ and $V_i$.
%, $U = \begin{bmatrix} U_1\\
%\vdots \\
%U_n \end{bmatrix}$, $V = \begin{bmatrix} V_1\\
%\vdots \\
%V_n \end{bmatrix}$, with $U_i, V_i \in \Real^{3 \times 3}$. 
Let $F=U V^T + V U^T$ and denote $F_{ij}=U_{i}V_{j}^{T}+V_{i}U_{j}^{T},~ i,j=1,\ldots,n$ and $F_i = U_i V^T + V_i U^T,~i=1,\ldots,n$. 

Assume that $rank(F_{ij})=2$ for $i \neq j$, and $F_{ii}=0_{3 \times 3}$, $rank(F_i) =3$ for $i=1,\ldots,n$ . Then it holds that either $\forall i\,rank(V_{i})=3,\,rank(U_{i})=2$ or that $\forall i~rank(V_{i})=2,\,rank(U_{i})=3$.
\end{lemma}
%  \begin{lemma}\label{lemma:xor}- For $U_{i},V_{i}$ as in eq. (2) it holds that
% either $\forall i\,rank(V_{i})=3,\,rank(U_{i})=2$ or that $\forall i\,rank(V_{i})=2,\,rank(U_{i})=3$
% \end{lemma}

\begin{proof}  First, since $\forall i~F_{ii}=0$, we have $\forall i ~U_{i}V_{i}^{T}$ is skew-symmetric $\Rightarrow rank(U_{i}V_{i}^{T})=2 \Rightarrow $ $rank(U_{i})\geq2$
and $rank(V_{i})\geq2$  (clearly $rank(U_i) \leq 3$ and $rank(V_i) \leq 3$). Let us check the different possible options. 
\begin{enumerate}
\item $\exists i$ such that $rank(U_i) = rank(V_i) =3 \Rightarrow \exists i$ such that $rank(U_i V_i^T) = 3$. However, this contradicts the observation that $\forall i~rank(U_{i}V_{i}^{T})=2$.

\item  $\exists i$ such that $rank(U_i) = rank(V_i) =2$. According to Lemma  \ref{lemma:common_null_space}, $\exists {\bf t} \in \Real^3$, such that $U_i^T {\bf t} = V_i^T {\bf t}=0 \Rightarrow F_i^T {\bf t} = (V U_i^T + U V_i^T) {\bf t} = 0$. However, this contradicts the full rank assumption over $F_i$.

\item  
Without loss of generality, we assume that 
\begin{align*}
rank(V_{1}) & =3,~rank(U_{1})=2\\
rank(V_{2}) & =2,~rank(U_{2})=3.
\end{align*}
By Lemma \ref{lemma:skew}, since $U_1 V_1^T$ is skew symmetric and $rank(V_1)=3, rank(U_1)=2$, we obtain that $T_1 = V_1^{-1}U_1$ is skew symmetric. From similar considerations $T_2 = U_2^{-1}V_2$ is skew symmetric. This yields 
\begin{align*}
F_{12} & = U_{1}V_{2}^{T}+V_{1}U_{2}^{T} \\
& =V_{1}T_{1}(-T_{2})U_{2}^{T}+V_{1}U_{2}^{T}\\
 & =V_{1}(-T_{1}T_{2}+I)U_{2}^{T}.
\end{align*}
Now, using the fact that $rank(V_1) = rank(U_2) =3$, we obtain  
\begin{equation}\label{eq:rank} rank(-T_{1}T_{2}+I) =rank(F_{12})=2. \end{equation}
In the next steps we show that $rank(-T_{1}T_{2}+I)$ is either 1 or 3, contradicting \eqref{eq:rank}. If it is full rank we are done. Otherwise, if $(-T_{1}T_{2}+I)$ is rank  deficient, then  
for any $v \in null(-T_{1}T_{2}+I)$ it holds that
\begin{align*}
(-T_{1}T_{2}+I)v & = 0\Rightarrow T_{1}T_{2}v = v\Rightarrow t_{1}\times(t_{2}\times v) = v. 
\end{align*}
Using the identity  
$a\times(b\times c) = b(a^{T}c)-c(a^{T}b) $, 
and the relation  $t_1^T v = 0$, we obtain
\begin{align*} 
t_{1}\times(t_{2}\times v) & =v \Rightarrow\\
t_{2}(t_{1}^{T}v)-v(t_{1}^{T}t_{2}) & =v \Rightarrow \\
-v(t_{1}^{T}t_{2}) & =v \Rightarrow \\
(t_1^T t_2) &= -1.
\end{align*} 
Now, the subspace defined by $\{ u \in \Real^3 | u^T t_1 =0\} $ is of dimension 2. However, as we show below it is contained in $null(-T_{1}T_{2}+I)$, \yk{only if $t_1^Tt_2=-1$ otherwise the nullspace is empty} contradicting \eqref{eq:rank}. Indeed, 
\begin{align*}
(-T_{1}T_{2}+I)u & = \\ 
-t_1 \times (t_2 \times u) +u & = \\
 -t_2(t_1^T u) + u(t_1^T t_2) + u & = 0
 \end{align*}
\end{enumerate}
$\Rightarrow$ either $\forall i\,rank(V_{i})=3,\,rank(U_{i})=2$ or that $\forall i\,rank(V_{i})=2,\,rank(U_{i})=3$.
\end{proof}

With respect to the last Lemma note that, $rank(F_i) = 3 \Leftrightarrow rank(F_i^T) = 3 \Leftrightarrow \text{dim}(null(F_i^T)) = 0 \Leftrightarrow \nexists {\bf t} \in \Real^3$ s.t $F_i^T {\bf t} = 0 \Leftrightarrow \nexists {\bf t} \in \Real^3$ s.t. $\forall j F_{ji} {\bf t}=0$. \ag{maybe explain more since it enforce non collinearity}
